# Supplementary material for: Higgs-boson production at the Photon Collider at TESLA
Source: arXiv:hep-ph/0503295 source file (2005-03-31)
Supplement: Supplementary file 1 [file appendix_gagaQQg_old.tex]

\chapter{Process $\gagaQQg$  \label{app_compnlolo}} 

%
%\input{Sections/
%As it is well known, 
%
NLO corrections to the cross section for the background process $\gagaQQ$
are large (see \eg \cite{JikiaAndTkabladze, MellesStirlingKhoze}).
%
Whereas the LO background  is strongly suppressed for  a  \( J_{z}=0 \) contribution, 
this suppression is much weaker for the  higher order contributions
due to the additional  gluon emission or exchange in the final state. 
%
As an example, we show in Fig. \ref{fig:Background_NLO_to_LO_ratio}
 the  ratios of the corresponding NLO and  LO results for the $W_{rec}$
distribution,  for the 
process $\gagabbg$, for different
values of \( N_{\rm jets} \) and \( J_{z} \). 
%
In each case  one observes large 
differences between the NLO and LO results, both in the shape and in the
normalization. 
%
As the precise determination of the background shape
is crucial for a reliable  estimation of the Higgs-boson  width, we conclude
that a rescaling of the LO estimates cannot be considered 
as a substitute of the full NLO background analysis.
%
%
The NLO background contribution
is  approximately two times larger than the LO one.
%
This is mainly due to the $J_z=0$ component, 
which is strongly suppressed in the LO case; however in the case of NLO it gives
a large contribution,
especially pronounced in the high-$\Wgaga$ part of the signal peak.
%

%%%
\pnfig{h}{9cm}{Plots/nlo_to_lo_ratio_for_bbg.eps}{fig:Background_NLO_to_LO_ratio}{
Ratio of the NLO to  LO results for the reconstructed invariant mass $W_{rec}$
distribution for the background process  $\gagabbg$.}
%%%
